# Supplementary material for: From flat to tilted: gradual interfaces in organic thin film growth
Source: arXiv:2003.07771 ancillary file (2020-03-17)
Supplement: Supplementary file 1 [file supporting_information.pdf]

# Supplementary Information to "From Flat to Tilted: Gradual Interfaces in Organic Thin Film Growth"

Laura Katharina Scarbath-Evers,[‡a] René Hammer,[b‡] Dorothea Golze,[c] Martin Brehm,[a] Daniel Sebastiani,[a] and Wolf Widdra [*b]

## Large-scale STM image of the $\alpha$-6T monolayer

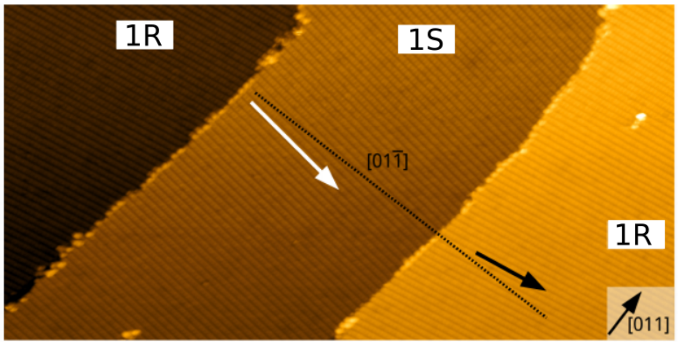


**Fig. S1** Large-scale STM image of the $\alpha$-6T monolayer on Au(100) (20 pA, 2.3 V, 80 K). The molecules adsorb completely flat in well ordered rows. Two domains, 1R and 1S, can be distinguished according to the direction of the molecular rows with respect to the [1$\bar{1}$0] direction. The direction of the molecular rows in the 1R and 1S domains is visualized by a black and white arrow, respectively.

Figure S1 depicts a large-scale STM image of a full monolayer of $\alpha$-6T on three different substrate terraces. We observe the growth of flat-lying, well-ordered molecular rows in densely packed monolayer domains, which are denoted as 1S (only S-enantiomeric molecules) and 1R (only R-enantiomeric molecules), see section 2.1 in the manuscript. In both domains, the long molecular axis is parallel to the [110] direction and almost perpendicular to the growth direction of the molecular rows. This orientation originates from the corrugation of the underlying substrate: for Au(100) the surface reconstruction leads to the formation of reconstruction rows that run in [110] direction. An arrangement of the molecules with their long molecular axis parallel to the reconstruction rows is energetically preferred, see also Ref. 1. On Ag(100), which is unreconstructed, $\alpha$-6T adopts a majority structure in which the molecules also arrange in densely packed rows. Unlike for the Au(100) substrate, the growth direction of the molecular rows is not approximately perpendicular to the [110] direction, but encloses an angle of 57° with the [110] direction.[2] The structural differences between the monolayer on Au(100) and Ag(100) can be explained by the missing reconstruction of the Ag(100) surface.

## Molecular orbitals of thiophene

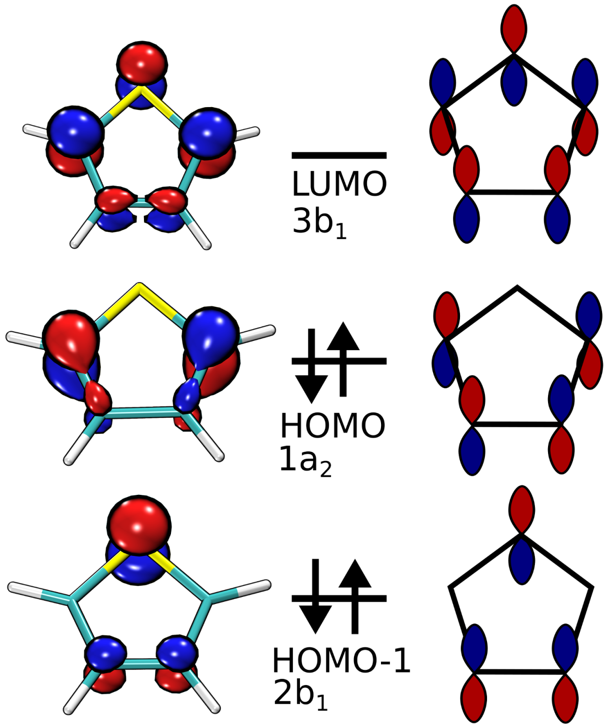


**Fig. S2** Left: Computed LUMO, HOMO and HOMO-1 of thiophene. Right: Schematic of the of the molecular orbitals and symmetry labels showing that the $\pi$ electrons of the sulfur do not contribute to the HOMO. Red and blue indicate different phases of the wave function.

[a] *Martin-Luther University Halle-Wittenberg, Institute of Chemistry, Halle/Saale, Germany*
[b] *Martin-Luther University Halle-Wittenberg, Institute of Physics, Halle/Saale, Germany*
[c] *Department of Applied Physics, Aalto University School of Science, FI-00076 Aalto, Finland*
‡ Both authors contributed equally
# *Current affiliation: Schrödinger Gmbh, Q7 23, 68161 Mannheim, Germany*
* Email: wolf.widdra@physik.uni-halle.de

**Table S1** Eigenvalues obtained from KS-DFT using the PBE0 functional and quasiparticle energies from $G_0W_0$ using PBE0 for the underlying DFT calculation. For $G_0W_0$, basis set extrapolated values are shown. All values in eV.

| Level | KS-DFT | $G_0W_0$ |
|---|---|---|
| LUMO | −0.19 | 1.05 |
| HOMO | −6.86 | −9.09 |
| HOMO-1 | −7.20 | −9.49 |
| HOMO-LUMO gap | 6.67 | 10.13 |

In the following we will discuss the electronic structure of $\alpha$-6T starting from a single thiophene. Figure S2 shows a plot of the highest molecular orbital (HOMO), the next lower orbital (HOMO-1), and the lowest unoccupied molecular orbital (LUMO) of a single thiophene molecule. All three MOs have $\pi$ character. The $p$ orbitals of the sulfur contribute to the HOMO-1, but not to the HOMO. The latter is only formed from the $p$ orbitals of the carbon atoms. The symmetry of the HOMO, HOMO-1 and LUMO is retained in the oligomer.[3] Our experimental and the computational STM images of $\alpha$-6T@Au(100) are obtained at a bias voltage that probes only the HOMO. We find indeed that the HOMO has no density at the sulfur and observe droplet-shaped lobes that can be assigned to the aromatic carbon atoms of $\alpha$-6T.

The energy that correspond to the HOMO, HOMO-1 and LUMO are presented in Table S1, comparing eigenvalues from KS-DFT and quasiparticle energies from $G_0W_0$. For the occupied states, the ionization potentials (IP) can be assigned to the negative of the DFT eigenvalues ($\varepsilon^{\mathrm{DFT}}$) or the quasiparticle energies ($\varepsilon^{\mathrm{QP}}$), IP$= -\varepsilon^{\mathrm{DFT/QP}}$. Compared to $G_0W_0$, DFT underestimates the IPs and yields too small LUMO energies and band gaps. However, the PBE0 functional yields the correct energy ordering of the two first occupied orbitals (HOMO, HOMO-1) and the LUMO.

The following computational settings are used for the $G_0W_0$ calculation: The PBE0 functional has been employed for the preceding DFT calculation ($G_0W_0$@PBE0). The $GW$ self-energy has been obtained from a full-frequency integration using the analytic continuation. For the analytic continuation a Padé approximant[4] with 16 parameters is used in combination with a Clenshaw-Curtis[5] with 1000 grid points. The QP equation is solved iteratively. The $G_0W_0$ calculations are performed with the CP2K program packages using the $N^4$ scaling implementation,[6] where $N$ refers to the system size. The $G_0W_0$ energies are extrapolated to the completed basis set limit accounting for the slow convergence with respect to basis set size characteristic for correlated electronic structure methods. The extrapolated results are computed from correlation consistent Gaussian basis sets of quadruple and quintuple$-\zeta$ quality (cc-QZVP and cc-5ZVP) by a linear regression against the inverse of the total number of basis functions, see Ref. 6 for details on the basis sets.

## Computed bilayer structures

The upper panel of Figure S3 depicts the computed bilayer structures found by our structure search in which we started from different initial position to avoid being trapped in a local minimum. The bilayers with a staggered configuration (III) are observed in experiment. For the 2S@1S bilayer the structure optimizations yield in addition an equally tilted arrangement (II), which is equal in energy.

For the 2R@1R structure, we found also another staggered structure III which was slightly higher in energy ($\approx 2.5\,\mathrm{kJ\,mol^{-1}}$ per molecule) than the one discussed in the main text and which has smaller shifts ($\Delta_{\mathrm{LMA}} \approx 0.8\,\mathrm{Å}$, $\Delta_{\mathrm{lat}} \approx 2\,\mathrm{Å}$), but otherwise exhibits similar tilt angles and overall the same qualitative structural behaviour as the lowest energy structure III .

The tilt angles were calculated based on the average height difference between the sulfur atoms of two adjacent thiophene units. Since the outermost thiophene units of the second-layer molecules are strongly bent downwards to increase the interactions with the gold surface (see Figure S4), the first two thiophene units were omitted from the analysis.

The lower panel of Figure S3 depicts the corresponding calculated STM images of the three structures. The STM of structure II shows indeed a unit cell comprising only one $\alpha$-6T molecules, i.e. the STM pattern of two consecutive molecules is the same, while it is reverted for structure III. In section "Molecular orientation in the second layer" in our manuscript, we compare the experimental STM image with the HOMO density of the molecule (i.e. the computed STM of the gas phase molecule). Such a comparison is possible if the electronic states of surface and molecule are electronically decoupled and if the bias voltage is chosen such that only the highest molecular orbitals fall within the energy range of $E_{\mathrm{Fermi}}$-$E_{\mathrm{Fermi}} + e \cdot V_{\mathrm{bias}}$. In that case the measured local density of states should exhibit the same symmetry as the HOMO density of the isolated molecule. In our case the first layer sufficiently decouples the molecular electronic states and that from the surface. Moreover, we performed scanning tunneling spectroscopy measurements which gave us the HOMO energy of the molecules in the second layer and allowed us to choose the bias voltage of the STM measurement accordingly.

## Interaction and adsorption energies

**Table S2** Adsorption and interaction energy for $\alpha$-6T on Au(100) and two stacked $\alpha$-6T molecules as model system for the interaction between a molecule in the first layer and in the second layer.

| System | E [$\mathrm{kJ\,mol^{-1}}$] |
|---|---|
| 2 $\alpha$-6T stacked | 47 |
| $\alpha$-6T@Au(100) (full DFT)[7] | 417 |
| $\alpha$-6T@Au QM/MM | 519 |

Figure S4 depicts a structural snapshot of the computed 2S@1S bilayer structure; for a better visualization only one molecular row of the second layer is shown. The shift along the LMA is clearly visible and enables a downward bent configuration of the first thiophene unit, as highlighted by a red rectangle. Such a downward bent configuration is favorable since it increases the interactions between the molecules in the second layer and the surface, which exceed the molecule-molecule interactions by far: the molecule-

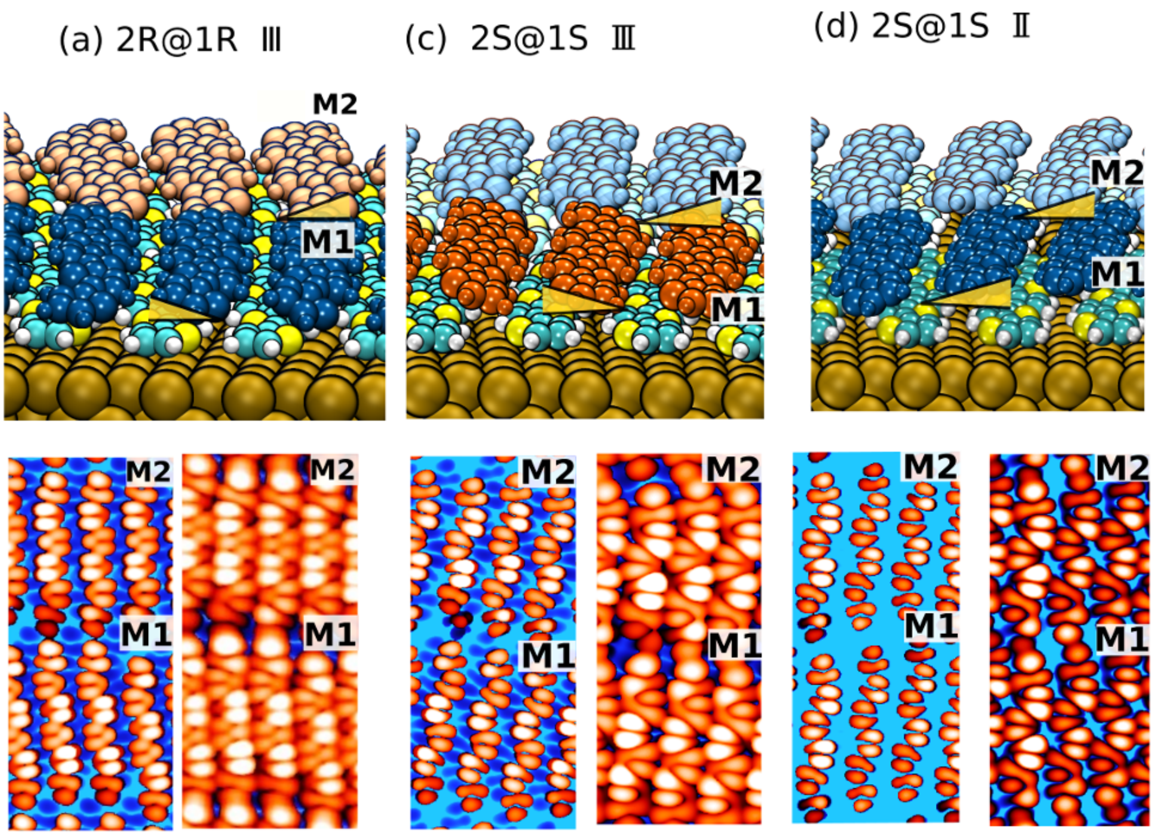


**Fig. S3** Calculated STM images of the staggered 2R@1R and 2S@1S structures (structure III) as well as of the equally tilted 2S@1S structure II that was not observed experimentally.

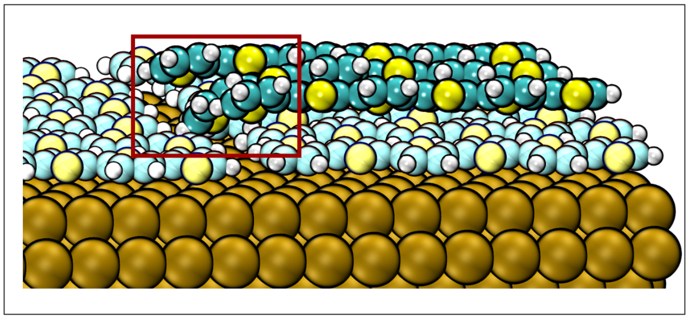

**Fig. S4** Structural snapshot of one molecular row in the second layer of the 2S@1S structure. It can be seen that the first thiophene unit of the molecules in the second layer is bent towards the surface.

molecule interaction energy is about 10 times smaller than the adsorption energy, see Table S2.

The interaction energy is computed at the DFT level and defined as follows

$$E_{\text{int}} = E_{\text{6T}-\text{6T},\text{opt}} - 2 \cdot E_{\text{6T},\text{gp opt}}, \qquad (1)$$

where $E_{\text{6T}-\text{6T},\text{opt}}$ is the energy of the optimized $\alpha$-6T dimer and $E_{\text{6T},\text{gp opt}}$ is the energy of the optimized $\alpha$-6T molecule in the gas phase. The counterpoise correction[8] has been used to account for the basis set super position error (BSSE). The adsorption energy is defined as

$$E_{\text{ads}} = E_{\text{opt}}^{\text{mol at Au}} - E_{\text{opt}}^{\text{mol,gp}} - E_{\text{opt}}^{\text{Au,clean}}, \qquad (2)$$

where $E_{\text{opt}}^{\text{mol at Au}}$ is the energy of the optimized molecule-surface complex, $E_{\text{opt}}^{\text{mol,gp}}$ is the energy of the optimized molecule in gas phase and $E_{\text{opt}}^{\text{Au,clean}}$ is the energy of the pristine Au(100) surface.

So far, no experimental values are available for the adsorption energy of $\alpha$-6T on gold. However, the adsorption energy of a single thiophene molecule on gold has been derived from desorption spectroscopy experiments[9–11] applying the Redhead equation.[12] They obtained adsorption energies lie in the range of $51\,\text{kJ mol}^{-1} - 75\,\text{kJ mol}^{-1}$. Calculations of the adsorption energy of thiophene on gold at the DFT level of theory[13] yield adsorption energies of $74\,\text{kJ mol}^{-1}$, in agreement with experimental values. We computed the adsorption energy of $\alpha$-6T on Au(100) with a similar full-DFT setup.[7] The result is given in Table S2.

## STM images of the third layer

High-resolution STM images of 2 molecules adsorbed on top of the 2R bilayer are presented in Figure S5 (a) and (b). One molecule appears as five bright protrusions from which three are elliptically shaped (protrusion1, protrusion 3, protrusion 5) while two are droplet-shaped (protrusion 2, protrusion 4). Additionally we observe several darker protrusions for molecule 1. According to the height profile depicted in Figure S5, they are $\approx 1.2$Å lower in

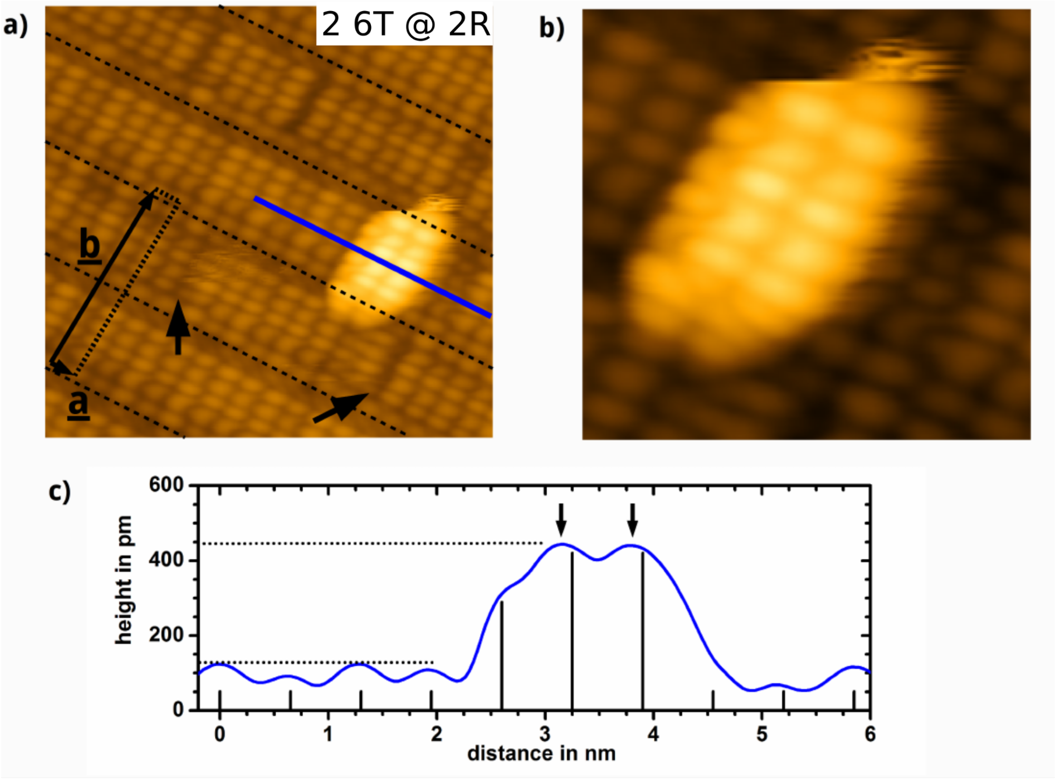


**Fig. S5** (a) Large-scale STM image of two molecules on a 2R bilayer. Dotted lines indicate the separation between different molecular rows. (b) Expanded scale image of the two molecules on top of a 2R bilayer. (c) Height profile along the blue line in (a). The maxima are indicated by black vertical lines.

height. This finding is a strong indication that the two molecules in the beginning third layer are tilted as well.

Further information for the interpretation of Figure S5 (a) and (b) can be obtained from Figure S6, which depicts the STM image of a flat lying molecule on top of a minority bilayer structure measured at a bias voltage of $-2\,\mathrm{V}$. This minority structure consists of small, two-dimensional island of flat lying molecules on top of the monolayer. It is formed only for a coverage smaller than 2 layers and is therefore not relevant for the gradual growth mechanism over several full layers discussed in the paper. However, the comparison of the corresponding protrusion pattern to the tilted structure yields valuable insights. The molecule in the third layer shows the following protrusion pattern: Three elliptic protrusions are located at the right-hand side of the LMA, and another three at the left-hand side. Additionally, we observe two large, s-shaped protrusions, which are marked by red arrows; for better visibility, one of the s-shaped protrusion is also indicated by a black, dashed line. Looking at Figure S6 (b), we see that for an anti-clockwise rotation of the molecule, the three elliptic protrusions on the right side of the LMA will dominate the STM image. Moreover, the s-shaped protrusions will appear droplet-shaped. Likewise, for a clockwise rotated molecule, schematically shown in Figure S6 (c), the three elliptic protrusions on the left side of the LMA are much closer to the tip and will therefore dominate the image. The s-shaped protrusions will again appear droplet shaped, however these droplets will be 180° rotated compared to the clockwise rotated molecule in Figure (b). Taking again a closer look at Figure S5 (a) and (b), we observe, that the droplet-shaped protrusions for molecule I and II look identical, thus both molecules are tilted in the same direction. The droplet-shaped protrusions of the molecules in the underlying molecular row, however, appear 180° rotated compared to those of molecule I and II. This observation indicates that the 2 molecules in the beginning third layer are tilted in opposite direction with respect to the molecules in the underlying molecular row, leading to a AB-like structure.

A high-resolution STM image of a fully-formed third layer is depicted in Figure S7. The molecular rows appear alternately darker and brighter which suggests a defect-like incorporation of the vertical shift $\Delta z$ which is also present in the bulk structure.

## Validation of the QM/MM model

The interactions between molecules and surface are described in our QM/MM model at the MM level of theory. The electrostatic interactions are accounted for by the image charge formulation and require no parametrization. However, the dispersion interaction and Pauli repulsion are described by force fields. We use a Lennard-Jones potential and assess its accuracy by comparing the adsorption energy obtained from the QM/MM model to full-DFT calculations.

The Lennard-Jones parameter can be obtained from different combination rules, which have a significant impact on the accuracy of our model. The well-known Berthelot mixing rules which

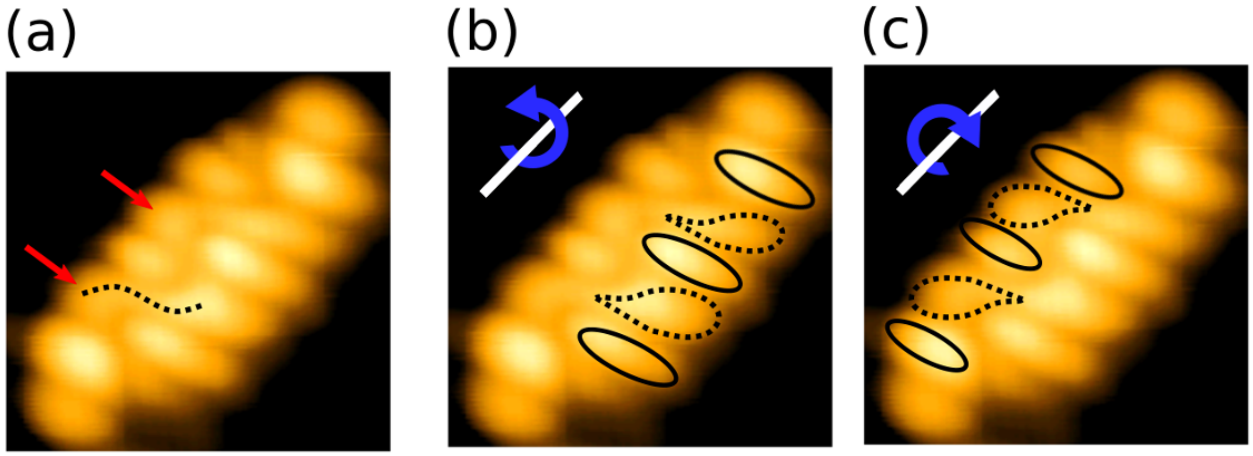


**Fig. S6** (a) Orbital-resolved STM image of a flat lying molecule on top of a minority bilayer structure measured at $-2\,\mathrm{V}$. Schematic illustration of an anti-clockwise (b) and clockwise (c) rotation of the molecule (the STM image is the same as in (a)).

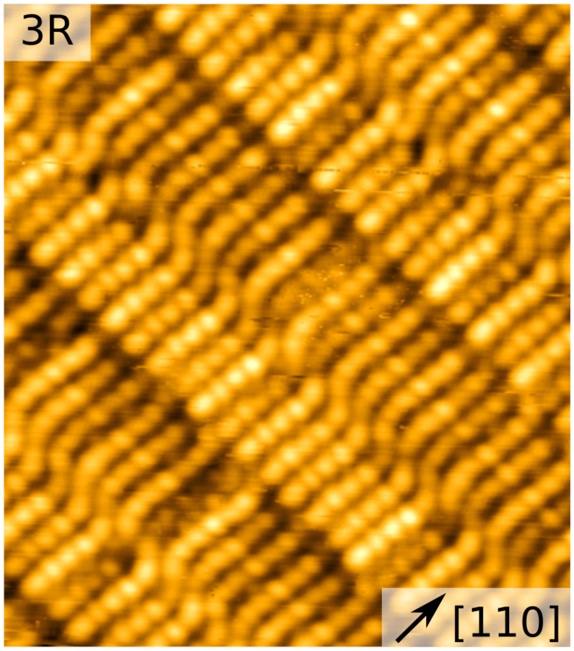


**Fig. S7** Large scale STM image of a full third layer ($-1.35\,\mathrm{V}$, $25\,\mathrm{K}$, $5\,\mathrm{pA}$). The molecular rows appear alternately darker and brighter indicating the incorporation of a vertical shift, $\Delta z$, between two alternately tilted rows, similar to the bulk structure.

are adequate for elements of the first two rows fail to describe interactions with heavy elements beyond the first and second row in terms of overestimating the non-covalent interactions.[14] Indeed, we find that employing only the Berthelot rules leads to an overestimation of the adsorption energy of a single thiophene molecule of over 50 % ($113\,\mathrm{kJ\,mol^{-1}}$ vs. $74\,\mathrm{kJ\,mol^{-1}}$ from full-DFT calculations.[13]) The mathematically derived Waldman-Hagler rules were already successfully applied to describe the interaction between atoms with largely different $Z$ numbers in a similar system as ours.[15] It was further suggested to use the Berthelot combination rules only for hydrogen and employ the Waldmann-Hagler rules for all heavy atoms.[16] Following this approach, we obtain an adsorption energy of $\approx 88\,\mathrm{kJ\,mol^{-1}}$ for one thiophene on a hexagonal Au surface which is only $\approx 20\,\%$ higher than the results from full DFT calculations. Similarly, with this approach the adsorption energy of a single $\alpha$-6T molecule amounts to $519\,\mathrm{kJ\,mol^{-1}}$ which is roughly 25 % larger than the adsorption energy calculated using a full-DFT setup ($417\,\mathrm{kJ\,mol^{-1}}$, see Table S2) The corresponding parameters are given in Table S3.

With a deviation of only 25%, we still obtain qualitatively the correct results for the adsorption of the monolayer. Our QM/MM model predicts in agreement with experiment flat-lying molecules assembled in rows. Relevant for the growth of the bilayer is the correct description of the molecule-molecule interaction, which is 10 times smaller than the adsorption energy, see Table S2. The molecule-molecule interactions are described at the DFT level using a hybrid functional and are therefore of high accuracy.

**Table S3** Lennard-Jones parameter for the $\alpha$-6T-Au interaction using the Waldmann-Hagler combination rules for the Au-S/Au-C parameter and the Berthelot combination rules for the Au-H parameter.

| | $\varepsilon$[kcal mol$^{-1}$] | $\sigma$[Å] |
|---|---|---|
| Au-S | 0.802 | 3.244 |
| Au-C | 0.424 | 3.244 |
| Au-H | 0.398 | 2.52 |

## $\alpha$-6T bulk structure

We performed a cell optimization of the $\alpha$-6T bulk structure using the PBE functional and D3 approximation and compared the cell vectors of the relaxed structure with the experimentally obtained cell vectors. We find, that the deviations are not larger than 1 %.

**Table S4** Comparison of the computed and experimental cell vectors of the $\alpha$-6T bulk structure. Computational values are obtained at the KS-DFT level using the PBE functional.

| vector | 6T bulk exp. | 6T bulk comp. | Δ [%] |
|---|---|---|---|
| $|a|$ | 44.708 | 45.276 | 1.3 |
| $|b|$ | 7.851 | 7.915 | 0.8 |
| $|c|$ | 6.029 | 5.95 | 1.3 |

## Notes and references


1 A. Höfer, K. Duncker, M. Kiel, S. Wedekind and W. Widdra, *Phys. Rev. B*, 2011, **83**, 075414.

2 K. Duncker, M. Kiel, A. Höfer and W. Widdra, *Phys. Rev. B*, 2008, **77**, 155423.

3 R. Telesca, H. Bolink, S. Yunoki, G. Hadziioannou, P. T. Van Duijnen, J. G. Snijders, H. T. Jonkman and G. A. Sawatzky, *Phys. Rev. B*, 2001, **63**, 155112.

4 H. J. Vidberg and J. W. Serene, *J. Low Temp. Phys.*, 1977, **29**, 179–192.

5 J. P. Boyd, *J. Sci. Comput.*, 1987, **2**, 99–109.

6 J. Wilhelm, M. Del Ben and J. Hutter, *J. Chem. Theory Comput.*, 2016, **12**, 3623–3635.

7 L. K. Scarbath-Evers, M. Todorović, D. Golze, R. Hammer, W. Widdra, D. Sebastiani and P. Rinke, *Phys. Rev. Materials*, 2019, **3**, 011601.

8 S. Boys and F. Bernardi, *Mol. Phys.*, 1970, **19**, 553–566.

9 S. M. Wetterer, D. J. Lavrich, T. Cummings, S. L. Bernasek and G. Scoles, *J. Phys. Chem. B*, 1998, **102**, 9266–9275.

10 G. Liu, J. A. Rodriguez, J. Dvorak, J. Hrbek and T. Jirsak, *Surf. Sci.*, 2002, **505**, 295 – 307.

11 A. Nambu, H. Kondoh, I. Nakai, K. Amemiya and T. Ohta, *Surf. Sci.*, 2003, **530**, 101 – 110.

12 P. Redhead, *Vacuum*, 1962, **12**, 203 – 211.

13 R. J. Maurer, V. G. Ruiz, J. Camarillo-Cisneros, W. Liu, N. Ferri, K. Reuter and A. Tkatchenko, *Prog. Surf. Sci.*, 2016, **91**, 72–100.

14 W. Song, P. J. Rossky and M. Maroncelli, *J. Chem. Phys.*, 2003, **119**, 9145–9162.

15 W. Janke, *Phys. Procedia*, 2015, **68**, 69 – 79.

16 A. Nikitin, Y. Milchevskiy and A. Lyubartsev, *J. Phys. Chem. B*, 2015, **119**, 14563–14573.
